# Supplementary material for: Power-Grid Controller Anomaly Detection with Enhanced Temporal Deep Learning
Source: arXiv:1806.06496 source file (2019-06-23)
Supplement: Supplementary file 1 [file appendix.tex]

\section*{Appendix}\label{sec:appendix}
\subsection*{A. Availability of HPCs}\label{sec:HPCavailability}
HPCs have been widely implemented on most commodity processors, include Intel, ARM and PowerPC. 

An Intel processor provides various CPU performance measurements in real-time in HPCs. It supports not only "core", but also "uncore", performance counters. Core refers to the processor, its general-purpose registers and its private caches. Uncore refers to the Level-2 (L2) or Level-3 (L3) cache shared between cores, the integrated memory controllers, and the Intel QuickPath Interconnect to the other cores and shared system components and the I/O hub. Examples of the core HPCs are the number of: instructions retired, elapsed core clock ticks, L2 cache hits and misses, L3 cache misses and hits, and the core frequency. Examples of the uncore HPCs are the number of: bytes read from memory controller(s), bytes written to the memory controller(s), and data traffic transferred by the Intel QuickPath Interconnect links.

There are also many performance event counters provided by an HPCs in an ARM processor. For example, the ARM Cortex-A series processor provides about 30 performance events, including the number of: Level-1 (L1) data cache refill events, or L1 instruction cache refill events, TLB (Translation Lookaside Buffer) refill events, all instructions executed, memory read/write instructions executed,  exceptions taken, exceptions returned, software changes of PC, branches executed, branches mis-predicted, external memory accesses, data memory accesses, and instruction cache accesses. However, only a given number of events, e.g. only 4 for Cortex-A8, can be read through the performance monitoring units at the same time.

\subsection*{B. Details on LSTM and CRBM}\label{sec:deepdetail}

We describe the detailed structures of LSTM, RBM and CRBM.

Figure \ref{fig:LSTM} shows the inner structure of LSTM \cite{LSTMIntro}. A basic LSTM cell has three gates that control information flow. The three gates are the forget gate $f_t$, input gate $i_t$ and output gate $o_t$. $f_t$ controls how much previous information remains in the memory. $i_t$ controls how much new information is stored in the memory, and $o_t$ controls how much information flows to the output. We define $x_t$ as the input vector. There are also two state vectors, i.e., cell vector $c_t$ and output vector $h_t$:

\begin{align}
f_{t}&= \sigma (W_{f}x_{t}+U_{f} h_{t-1}+b_{f})\\
i_{t}&= \sigma (W_{i}x_{t}+U_{i} h_{t-1}+b_{i})\\
o_{t}&= \sigma (W_{o}x_{t}+U_{o} h_{t-1}+b_{o})\\
c_{t}&= f_{t}.*c_{t-1}+i_{t} .* tanh(W_{c}x_{t}+U_{c} h_{t-1}+b_{c})\\
h_{t}&= o_{t}.*tanh(c_{t})
\end{align}
where $.*$ is element-wise multiplication and $\sigma$ is the sigmoid function.

\begin{figure}[h]
 \centering
  \includegraphics[width=\linewidth]{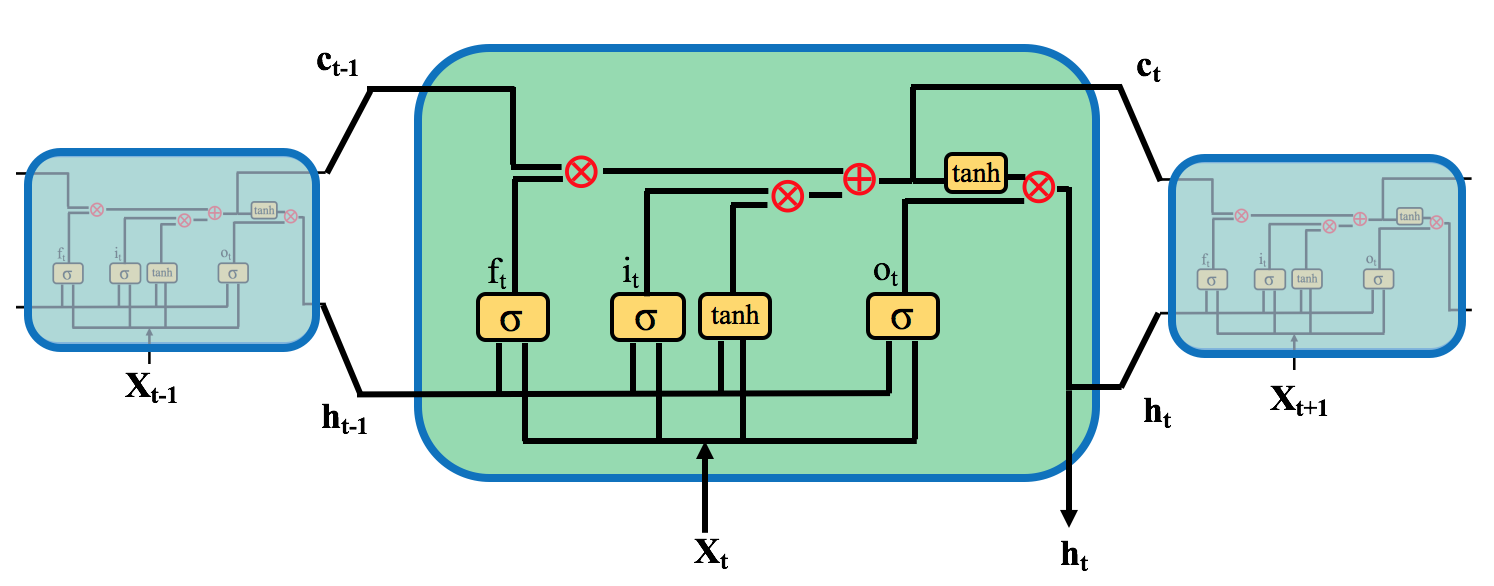}
  \caption{LSTM layers\cite{LSTMIntro}}
  \label{fig:LSTM}
\end{figure}

Restricted Boltzmann Machine (RBM) is another generative neural network which is able to learn a probability distribution. Figure \ref{fig:RBMandCRBM} left shows the basic structure of an RBM with m hidden units and n visible units \cite{fischer2012introduction}. Both hidden and visible units can only take values of zeros and ones. The probability of taken zeros and ones are given by the following equations (H denotes hidden units and V denotes visible units):

\begin{align}
p(H_i = 1 | v) &= \sigma(\sum_{j=1}^{m} w_{ij}v_{j} + c_{i})\\
p(V_j = 1 | h) &= \sigma(\sum_{i=1}^{n} w_{ij}h_{i} + b_{j})
\end{align}

where $\sigma$ is a sigmoid function. For RBM which takes real value inputs, the model can be extended to:

\begin{align}
p(H_i = 1 | v) &= \sigma(\sum_{j=1}^{m} w_{ij}v_{j} + c_{i})\\
p(V_j| h) &= N(b_{i} + \sum_{i=1}^{n} w_{ij}h_{i}, 1 )
\end{align}

where $N(\mu, \sigma)$ is a Gaussian function. Contrastive Divergence (CD) is a widely used approximation algorithm for training the RBM \cite{carreira2005contrastive}.

\begin{figure}[h]
 \centering
  \includegraphics[width=\linewidth]{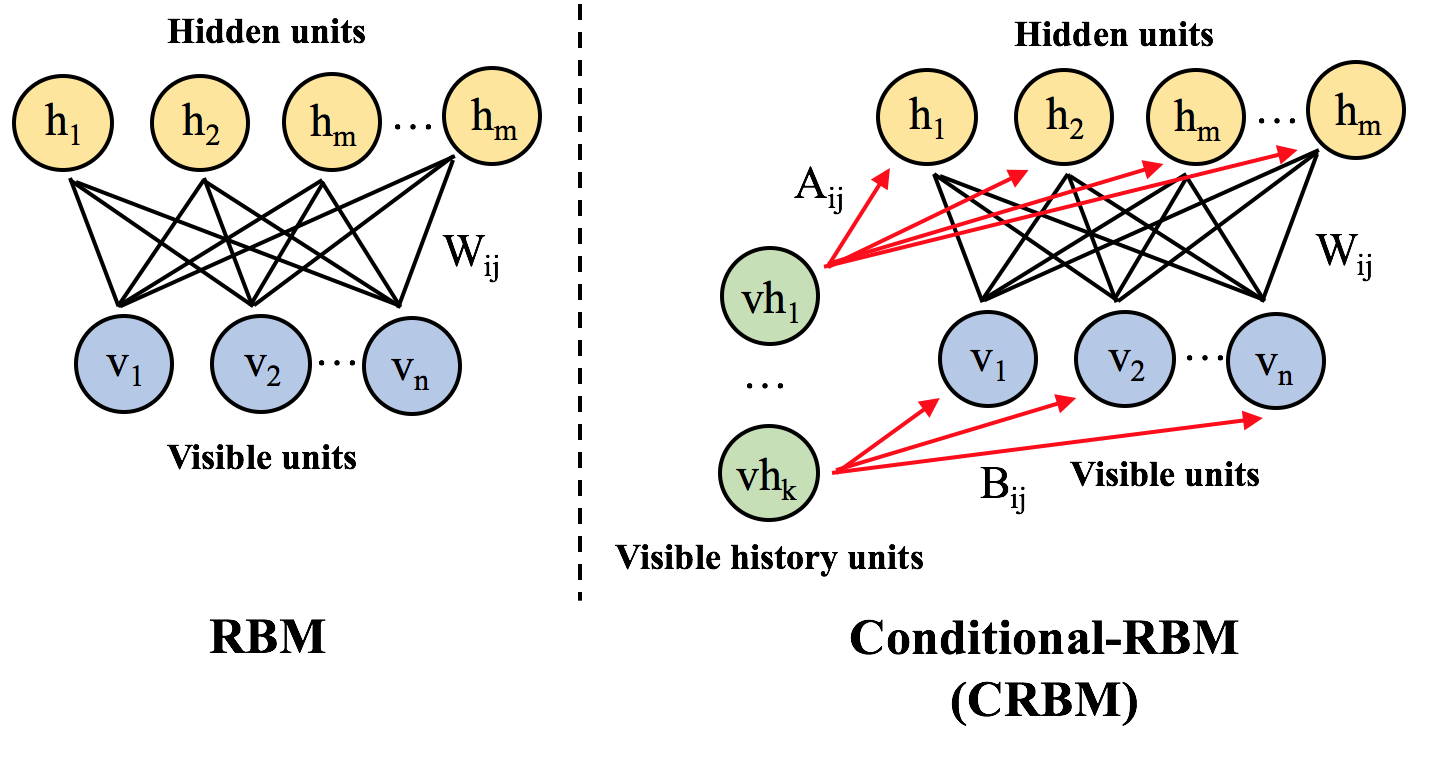}
  \caption{Left: The undirected graph of an RBM with m hidden and n visible variables \cite{fischer2012introduction}. Right: Conditional-RBM introduces history into RBM.}
  \label{fig:RBMandCRBM}
\end{figure}

However, the vanilla RBM does not consider any temporal information and thus is not feasible to be used as the predictor. Conditional RBM (CRBM) \cite{taylor2007modeling} is an extension of the original RBM by taking history information into consideration. Figure \ref{fig:RBMandCRBM} right shows the structure of a CRBM.  

\begin{align}
a_{i,t} &= a_{i} + \sum_{k} A_{ki}v_{k,<t}\\
b_{j,t} &= b_{j} + \sum_{k} B_{kj}v_{k,<t}
\end{align}

The effect of the history information on hidden units (and visible units) can be viewed as a dynamic bias $b_{j,t}$ ($a_{i,t}$) instead of $b_j$ ($a_i$) in the above equations \cite{taylor2011two}.
